# Supplementary material for: FARA: Future-aware Ranking Algorithm for Fairness Optimization
Source: arXiv:2305.16637 source file (2023-08-19)
Supplement: Supplementary file 1 [file appendix.tex]

\section{Theoretical Analysis}
\label{sec:theoreAnaly}
Here we provide theoretical analysis to help readers better understand the proposed algorithm. 
% \brutuscomment{I suggest we rename this subsection as "Discussions" and move 4.4.1 to Appendix. 4.4.2 and 4.4.3 seems reasonable discussion about FARA and 4.4.1 seems not that relevant.}
% \subsubsection\textbf{Exposure Error bound of Vertical Ranking} In this section, we will discuss how accurately vertical allocation can allocate the planing exposure  $\Delta E$. 
\subsection{Exposure Error bound of Vertical Ranking.} 
\label{sec:ExposureError}
Here we discuss the exposure allocation error bounds in Phase 2 of our algorithm, i.e, $|\Tilde{E}(d)-\Delta E(d)|$, in Algorithm~\ref{algo:VerticalAlloc}. 
% \subsection{Theoretical Analysis.}
We noticed that there are two possible scenarios of line 7-10 in Algorithm~\ref{algo:VerticalAlloc}: 

\textit{Scenario 1: There exists a $(rnk^*, sess^*)$ pair where $Set1 \cap Set2 =  \varnothing$}. If this happens, $(k_s, sess^*)$ will also have $Set1 \cap Set2 =  \varnothing$ since the size of $Set1$ and $Set2$ monotonically decrease  for lower rank of the same session. 
As $Set2$ is the set of unselected items for a session, we know that there are at least $|D|-k_s$ items in $Set2$, i.e., $|Set2|\ge |D|-k_s$.  If $Set1 \cap Set2 =  \varnothing$, those $|D|-k_s$ items are not in $Set1$.  In other words, there are at least $|D|-k_s$ items that satisfy $\Delta E(d)-\Tilde{E}(d)< P_{k_s}$.

% If this case exists, $Set1 \cap Set2 =  \varnothing$ also happens for lower ranks $(rnk^*+1, sess^*),(rnk^*+2, sess^*),...,(k, sess^*)$ since both $Set1$ and $Set2$ shrink for lower ranks of the same session and their intersection shrinks too. So $Set1 \cap Set2 =  \varnothing$ also happens for $(k, sess^*)$ and we consider the position $(k, sess^*)$ in the following. As the length of a ranked list is $k$, there should be $|D|-k$ items that haven't been selected before, $|Set2|=|D|-k$. $Set1 \cap Set2 =  \varnothing$ means at least those  unselected items are not in $Set1$. In other words, there are at least $|D|-k$ items that satisfy $\Delta E(d)-\Tilde{E}(d)\le \frac{p_{k}}{2}$. So vertical allocation can at least guarantee $|D|-k$ items to fulfill their exposure planing with error less than $\frac{p_{k}}{2}$. So vertical allocation can at least guarantee $|D|-k$ items to fulfill their exposure planing with error less than $\frac{p_{k}}{2}$.

\textit{Scenario 2: $Set1 \cap Set2 \neq \varnothing \: \forall (rnk, sess) $ pair}. Due to the margin $P_{rnk}$ in line~\ref{algo2:margin} of Algorithm~\ref{algo:VerticalAlloc}, $\Delta E(d)\ge \Tilde{E}(d) \: \forall d \in D$ should always hold if $Set1 \cap Set2 = \varnothing$ never happens.  By considering $\Delta E(d)\ge \Tilde{E}(d) \: \forall d \in D$ and the identity $\sum_{d\in D(q)}\Delta E(d)\equiv\sum_{d\in D(q)} \Tilde{E}(d)$, we would know that $\Delta E(d)= \Tilde{E}(d) \: \forall d \in D$, which means exposures are perfectly allocated according to $\Delta E(d)$.
% Let's consider the last position $(k, \Delta T)$. Before deciding the item for this position, the exposure left that have not been allocated is $p_k$, i.e., $p_k=\sum_{d\in D}(\Delta E(d)-\Tilde{E}(d))$. This means that there are most two items that satify $\Delta E(d)-\Tilde{E}(d)\geq \frac{p_{\textit{k_s}}}{2}$. This means that there are at least $|D|-2$ items that satisfy $\Delta E(d)-\Tilde{E}(d)\le \frac{p_{\textit{k_s}}}{2}$.

Since the size of documents is much greater than the number of items that users would examine, we have $|D|>>k_s$. Combing the two scenarios above, the vertical allocation in Algorithm \ref{algo:VerticalAlloc} can theoretically guarantee $\Delta E(d)-\Tilde{E}(d)\le P_{k_s}$ for at least $|D|-k_s$ items. Since $\Delta E(d)>> P_{k_s}$ when using our algorithm, we still claim that the vertical allocation in Algorithm \ref{algo:VerticalAlloc} can correctly allocate exposure.

\subsection{Solution to allocate $\Delta E^*$ is not unique.}
\label{sec:SolutionNotUnique}
In Appendix~\ref{sec:ExposureError}, we have proved that exposure can be correctly allocated.
The discussion in Sec.~\ref{sec:ExposureError} is independent of how we select item $d^*$ from the candidates set, and it does not need to be the most relevant one as we do in line ~\ref{algoline:priority} of Algorithm \ref{algo:VerticalAlloc}. So we could know that many ranklists can accurately allocate exposure and the solution is not unique.
\subsection{Why FARA can reach optimal effectiveness given exposure planning?} 
\label{sec:VerticalReason}
% In this section, we will give a theoretical analysis why vertical allocation can have better top rank effectiveness compared with Horizontal allocation given exposure planning.
Here we provide theoretical proof that vertical allocation, i.e., phase 2, can optimize effectiveness (\textit{aver-NDCG}) when exposure planning $\Delta E$ is given. 
Specifically, maximizing \textit{aver-NDCG}$@k_c$ in Eq.~\ref{eq:NDCG} is equivalent to
\begin{subequations}
\begin{align}
    \max \sum_{d\in D(q)}R(d)&  E@k_c(d) \label{eq:ignoreNorm} \\
\textit{s.t.}\quad \sum_{d\in D(q)}  E@k_c(d)&=Const.\label{eq:ExpoSumConstkc}\\
 0\le E@k_c(d)&\le \Delta E(d)\; \: \forall d\in D \label{eq:LessThanExpoPlanning}
\end{align}
\label{eq:proofOptim}
\end{subequations}
where normalization is ignored   in Eq.~\ref{eq:ignoreNorm}, the sum of top ranks exposure should be a constant in Eq.~\ref{eq:ExpoSumConstkc}, and the top ranks exposure should be less than the total exposure planning in Eq.~\ref{eq:LessThanExpoPlanning}. According to Rearrangement Inequality~\cite{hardy1952inequalities}, it is straightforward to know that \textit{aver-NDCG}$@k_c$, i.e., Eq.~\ref{eq:ignoreNorm},  can be optimized by letting item of greater relevance $R$ get more  exposure at top ranks, i.e., greater $E@k_c$. In other words, we should prioritize letting items of greater relevance $R$ fulfill their exposure planning $\Delta E$ at top $k_c$ ranks since $E@k_c$ is bounded in $[0,\Delta E]$. 
% When the total exposure planning is given, we need to decide how to distribute the total exposure at different ranks. 
By assuming that \textit{aver-NDCG} at higher ranks is more important~\cite{robertson1977prp}, we should maximize \textit{aver-NDCG}$@k_c$ before maximizing \textit{aver-NDCG}$@(k_c+1)$, $\: \forall\: 1\le k_c<k_s$.
% i.e., \textit{aver-NDCG}$@k_c$ is more important than \textit{aver-NDCG}$@(k_c+1) \: \forall\: 1\le k_c<k_s$.
% Given fixed exposure planning $\Delta E$, 
As we maximize \textit{aver-NDCG} from top to lower ranks, it is straightforward that the optimal way is to follow a greedy selection strategy to let an item of greater relevance $R$ fulfill its exposure planning $\Delta E$ at its highest possible ranks. In Algorithm \ref{algo:VerticalAlloc}, the proposed vertical allocation just follows the above greedy selection strategy to let item of greater relevance $R$ (line ~\ref{algoline:priority} in Algorithm \ref{algo:VerticalAlloc}) fulfill its exposure planning $\Delta E$ at the highest possible ranks (setting rank loops as the outer loop in ~\ref{algoline:loop1} and line ~\ref{algoline:loop2} of Algorithm \ref{algo:VerticalAlloc}).  Since the proposed vertical allocation in Algorithm \ref{algo:VerticalAlloc} follows the greedy selection strategy, it can reach optimal effectiveness at the top ranks.  

For a two-phase algorithm,  FARA's exposure planning $\Delta E^*$ is optimal by solving the QP problem in phase 1, and the final constructed ranklists are also optimal in phase 2. Since the two phases are both optimal, we claim that FARA is optimal.

\subsection{Effectiveness and fairness is fixed when $\Delta E$ is fixed.}
\label{sec:fixedEffFair}
Given the same exposure planning $\Delta E$, effectiveness (aver-NDCG$@k_s$) and fairness are fixed since we can substitute exposure planning $\Delta E(d)$  for $E^t@k_c(d)$ in Eq.~\ref{eq:NDCG} and substituting $\Delta E$  for $E$ in Eq.~\ref{eq:unfairness}, respectively. In other words, for any ranklist $\mathcal{B}^*$, as long as exposure planning $\Delta E$ can be accurately allocated in $\mathcal{B}^*$, the effectiveness and fairness are fixed.
